# Supplementary material for: Structured Training for Neural Network Transition-Based Parsing
Source: arXiv:1506.06158 source file (2015-06-19)
Supplement: Supplementary file 2 [file appendix.pdf]

# Structured Training for Neural Network Transition-Based Parsing

## Appendix

David Weiss   Chris Alberti   Michael Collins   Slav Petrov  
Google Inc  
New York, NY  
{djweiss,chrisalberti,mjcollins,slav}@google.com

### A Full Treebank Union Results

**Corpus details.** The corpora used in the Treebank Union setup are:

- English News Text Treebank: Penn Treebank Revised (LDC2015T13),
- OntoNotes version 5 (Hovy et al., 2006),
- English Web Treebank (Petrov and McDonald, 2012),
- Question Treebank (Judge et al., 2006) (updated and corrected),

yielding roughly  $\sim 90K$  training sentences in total.

The full test results including both UAS and LAS are included in Table 1.

### B Visualization of perceptron weights.

The perceptron weights  $\mathbf{v}$  from the  $\phi(x, c) = [\mathbf{h}_1 \mathbf{h}_2 P(y)]$  are visualized in the attached `weights_full.png`, and for  $\phi(x) = [P(y)]$  in `weights_Py_only.png`.

### References

- John Judge, Aoife Cahill, and Josef van Genabith. 2006. Questionbank: Creating a corpus of parse-annotated questions. In *Proc. ACL*, pages 497–504.
- Andre Martins, Miguel Almeida, and Noah A. Smith. 2013. Turning on the turbo: Fast third-order non-projective turbo parsers. In *Proc. ACL*, pages 617–622.
- Slav Petrov and Ryan McDonald. 2012. Overview of the 2012 shared task on parsing the web. Notes of the First Workshop on Syntactic Analysis of Non-Canonical Language (SANCL).
- Hao Zhang and Ryan McDonald. 2014. Enforcing structural diversity in cube-pruned dependency parsing. In *Proc. ACL*, pages 656–661.
- Yue Zhang and Joakim Nivre. 2011. Transition-based dependency parsing with rich non-local features. In *Proc. ACL-HLT*, pages 188–193.
- Bernd Bohnet and Jonas Kuhn. 2012. The best of both worlds: a graph-based completion model for transition-based parsers. In *Proc. EACL*, pages 77–87.
- Bernd Bohnet. 2010. Top accuracy and fast dependency parsing is not a contradiction. In *Proc. COLING*, pages 89–97.
- Eduard Hovy, Mitchell Marcus, Martha Palmer, Lance Ramshaw, and Ralph Weischedel. 2006. Ontonotes: The 90% solution. In *Proc. HLT-NAACL*, pages 57–60.

| Method                    | Beam | News         |              | Web          |              | Questions    |              |
|---------------------------|------|--------------|--------------|--------------|--------------|--------------|--------------|
|                           |      | UAS          | LAS          | UAS          | LAS          | UAS          | LAS          |
| <i>Graph-based</i>        |      |              |              |              |              |              |              |
| Bohnet (2010)             | n/a  | 93.29        | 91.38        | 88.22        | 85.22        | 94.01        | 91.49        |
| Martins et al. (2013)     | n/a  | 93.10        | 91.13        | 88.23        | 85.04        | 94.21        | 91.54        |
| Zhang and McDonald (2014) | n/a  | 93.32        | 91.48        | 88.65        | 85.59        | 93.37        | 90.69        |
| <i>Transition-based</i>   |      |              |              |              |              |              |              |
| *Zhang and Nivre (2011)   | 32   | 92.99        | 91.15        | 88.09        | 85.24        | <b>94.38</b> | <b>92.46</b> |
| Bohnet and Kuhn (2012)    | 40   | 93.35        | 91.69        | 88.32        | 85.33        | 93.87        | 92.21        |
| Our Greedy                | 1    | 92.92        | 91.21        | 88.32        | 85.41        | 92.79        | 90.61        |
| Our Perceptron            | 16   | <b>93.91</b> | <b>92.25</b> | <b>89.29</b> | <b>86.44</b> | 94.17        | 92.06        |
| <i>Tri-training</i>       |      |              |              |              |              |              |              |
| *Zhang and Nivre (2011)   | 32   | 93.22        | 91.46        | 88.40        | 85.51        | 93.74        | 91.36        |
| Our Greedy                | 1    | 93.48        | 91.82        | 89.18        | 86.37        | 92.60        | 90.58        |
| Our Perceptron            | 16   | <b>94.16</b> | <b>92.62</b> | <b>89.72</b> | <b>87.00</b> | <b>95.58</b> | <b>93.05</b> |

Table 1: Final Treebank Union test set results. We report LAS only for brevity; see Appendix for full results. For these tri-training results, we sampled sentences to ensure the distribution of sentence lengths matched the distribution in the training set, which we found marginally improved the ZPar tri-training performance. For reference, the accuracy of the Berkeley constituency parser (after conversion) is 93.29% / 91.66% News, 88.77% / 85.93% Web, and 94.92% / 93.45% QTB.
